# Supplementary material for: mHuBERT-147: A Compact Multilingual HuBERT Model
Source: arXiv:2406.06371 source file (2024-11-21)
Supplement: Supplementary file 1 [file appendix_table_per_validation.tex]

\begin{table*}
\centering
\begin{tabular}{lccccccccccc}
\toprule
                & \textbf{\begin{tabular}[c]{@{}c@{}}Average \\ PER\end{tabular}} & \textbf{es} & \textbf{fr} & \textbf{it} & \textbf{ky} & \textbf{nl} & \textbf{ru} & \textbf{sv} & \textbf{tr} & \textbf{tt} & \textbf{zh-HK} \\\midrule
Results from \cite{babu2021xls} & 6.5                                                             & 3.1         & 5.4         & 4.9         & 5.1         & 5.8         & 6.0         & 7.2         & 6.0         & 4.1         & 17.0           \\
Our setup       & 6.5                                                             & 4.1         & 5.4         & 5.3         & 4.9         & 5.3         & 6.0         & 8.0         & 5.7         & 3.7         & 17.0   \\\bottomrule       
\end{tabular}
\caption{Validation of our phoneme recognition setup described in \ref{appendix:impact:updates} using XLS-R 300M.}
\label{tab:persetup:validation}
\end{table*}
